# Supplementary material for: White Paper on Software Infrastructure for Advanced Nuclear Physics Computing
Source: arXiv:2501.00905 source file (2025-04-21)
Supplement: Supplementary file 1 [file AppendixReferenceMaterial.tex]

%=========================================================
\section{Miscellaneous material from workshop slides}

%------------------------
\subsection{Innovation and Stewardship}
\label{Sect:InnovationStewardship}

\subsubsection{Saturday bullets}

Saturday comments:

\begin{itemize}

\item Ron Soltz: Maintain $\rightarrow$ Steward

\item Ron Soltz: A new program is needed to build on the success of SciDAC and CSSI and foster collaborations among NP and data scientists to advance the science of the NSAC LRP.

\item Anonymous: See if it is beneficial to link to cybersecurity to emphasize the importance of sustained investments to ensure software integrity.

\item Gojko Vujanovic: Perhaps we can add here accelerated computing here, which allows to tackle larger-scale problems that are prohibitive otherwise.

\end{itemize}

\paragraph{K.Godbey}

Dedicated investments are needed to keep abreast of industry trends and best practices for the development of a sustainable software infrastructure for nuclear physics.

\paragraph{W. Hix}

SciDAC and CSSI have been invaluable in developing the software that allows nuclear physics to tackle important problems using high performance computing, by combining our expertise with that of computational science and applied mathematics. As research areas have matured, more are now are positioned to take advantage of these programs, therefore maximizing progress in nuclear physics would be facilitated by increased support for these programs.

The software developed by SciDAC, CSSI and other programs have a shelf life much longer than those programs duration. There is therefore a need in nuclear physics to maintain this software and make sure it functions optimally on new HPC systems as they become avaiable, in order to protect our prior investments.

The success in SciDAC + CSSI of the close collaboration of NP, CS + AM has taught us of the value of similar alliances as we seek to tackle forefront nuclear physics problems with the latest innovations in computing, most notably ML/AI and QIS.

\noindent{\bf UQ}  Uncertainty quantification with proper statistical treatment of correlated errors and error distributions is essential to take full advantage of recent advances in modeling and new experimental data. \\

Heterogeneous requirements: experiment
\begin{itemize}
\item Projects of different size have different requirements
\item Small (FRIB) $\rightarrow$ medium-sized (Jlab) $\rightarrow$ Large (EIC, LHC)
\item Independent (neutrino, project 8) vs hosted (LHC, EIC, FRIB, JLab,...)
\end{itemize}

Heterogeneous requirements: theory
\begin{itemize}
\item Projects of different size have different requirements
\item Single PI $\rightarrow$ US QCD
\end{itemize}

%------------------------
\subsection{Cross-cutting connections}
\label{Sect:CrossCuttingConnections}

Ron Soltz: Adding UQ bullet here,

\begin{itemize}
\item Uncertainty quantification with proper statistical treatment of correlated errors and error distributions is essential to take full advantage of recent advances in modeling and new experimental data.
\end{itemize}

Ensure Success for Software + Computing in NP: Encourage partnership between hosting institutions and experiments, between facilities, and between experiments.

Recent advances in techniques for model-to-data comparisons provide a compelling opportunity to forge new collaborations between experiment and theory to accelerate discovery in NP.

Uncertainty quantification with proper statistical treatment of correlated errors and error distributions is essential to take full advantage of recent advances in modeling and new experimental data. Closely connected to data preservation

Heterogeneous requirements: experiment
\begin{itemize}
\item Projects of different size have different requirements
\item Small (FRIB) $\rightarrow$ medium-sized (Jlab) $\rightarrow$ Large (EIC, LHC)
\item Independent (neutrino, project 8) vs hosted (LHC, EIC, FRIB, JLab,...)
\end{itemize}

Heterogeneous requirements: theory
\begin{itemize}
\item Projects of different size have different requirements
\item Single PI $\rightarrow$ US QCD
\end{itemize}

%------------------------
\subsection{Funding and Outreach}
\label{Sect:FundingOutreach}

Funding of Computing within projects/experiments

\begin{itemize}
\item Recognize software + computing and continuous R+D and as vital aspects of projects.
\item Support cross-cutting initiatives:
\item Expanded support for cross-cutting initiatives between experiment-theory in NHEP.
\end{itemize}

SciDac has been invaluable to connect NP with applied Math and CS, but we need a sustained effort

We need to do something similar to SciDac for QI, ML, accelerated computing, and advanced Nuclear Theory algorithms

We need to couple it with increased resources to make those ideas operational

Quantum: companies have significant more resources to support these activities, but we need to make sure that the resources do not disappear if the companies do

\begin{itemize}
\item Recognize that expertise outside NP is valuable to the Nuclear Physics enterprise
\item Avenues to promote multi-disciplinary opportunities
\item We need to be able to recruit the expertise that we need to achieve our goals, even if they are not NP
\item Applications where there is a specific need of this type should not be penalized
\end{itemize}

%------------------------
\subsection{Operations}
\label{Sect:Operations}

Development of common software ecosystems
\begin{itemize}
\item Computing centers that lower the barriers of entries
\item Host information on available software
\end{itemize}

Software lifecycle plan should be explicitly mentioned in funding opportunity announcements, perhaps as a part of the data management plan, with associated mechanisms to fund that plan

Software development/stewardship funding awards for theory-experiment collaborations should also incorporate computing allocations sufficient to the scientific need.

Markus: Experiments have been drivers for common software and common software ecosystems. This should be fostered and strengthened.

Eric Lancon: Software development should be considered as part of operation (which is not currently).

%------------------------
\subsection{Workforce and Community}
\label{Sect:Workforce}

\subsubsection{Saturday text}

\subsubsection{WG bullets and discussion}

Workforce Stewardship:
\begin{itemize}
\item Career support, career path, career opportunities essential for building work force.
\item Training essential.
\end{itemize}

Make possible long term positions for NP computing experts to maintain and develop codes 
We need a pot of money to support experts (students who have interest in computation can see a career path)

\begin{itemize}
\item Importance of sharing resources for training (repository with videos etc. to hit a large group of people + more targeted training (hackatons, schools))
\item Partnerships with industry are beneficial to the NP program (training of students)
\item Projects should promote workforce development for research computing and data science in addition to developing career pathways for young scientists in theory and experiment.
\end{itemize}

Self-replicating meeting: an annual meeting of this kind, bringing together all elements of the US NP community and agency reps, would be highly beneficial
\begin{itemize}
\item Communication, sharing of information
\item  new scientific connections
\item  Adjacent to October DNP meeting to minimize travel costs…?
\end{itemize}

Kyle: Not sure how best to message this, but funds to support pedagogy and community resources would be a great catalyst for innovation and lowering the barrier to doing great science. Right now we do this, primarily, in our spare time or through limited, targeted programs at the NSF. I would like to see some encouragement to make every proposed project reproducible in some way.

%------------------------
\subsection{Data Physicist}
\label{Sect:DataPhysicist}

Data Physics: Qualitatively New Distinction
New career title/job description: Data Physicist
New funding path within FAs for the new type (DP) proposals.

Projects should support funding in research computing and data science such as seeding permanent positions (similar to NP Theory Topical Collaborations) in research computing and data science

Text should focus on recognition
Flight risk

Closely connected to workforce bullet

Ron comment: What is the practical utility of this term?  Is there any benefit to defining a discipline that applies data science tools to physics problems, regardless of sub-field?  How does that differ from a data scientist who collaborates with physicists or a domain physicist in HEP/NP/BES/FES who works with data scientists?

Kyle comments:
\begin{itemize}
    \item For a broader dive into the term: https://www.aps.org/apsnews/2023/10/rise-of-data-physicist
    \item It is a little blurry, but I think it's an attempt to standardize a term for those that chronically work at boundary. In principle they could be put into either camp or classification you mentioned, but it's a marketing push and a way to make it a viable career path and to have a little continuity in collaboration.
    \item For purposes of the bullets, we probably want to pull this into our bullets on workforce and community
\end{itemize}

Loren comment: There is value in collaborating with data scientists who are physicists. My understanding is the title captures this need. Perhaps we don't need a new term but can use it as shorthand for now to capture this need.

%------------------------
\subsection{Data Preservation}
\label{Sect:DataPreservation}

\subsubsection{Saturday discussion}

Need to define “data”; “has longevity”; bits that someone took the effort to generate that need to be preserved (Eric comment: "into the data mgt plan")

Make connection to ASCR expertise; Nuclear data @BNL;...

Preserve derived data (shell model configs)

Centralization or heterogeneous? (At least a common web page etc)

Not for free - needs effort/support

FAIR standards

Data preservation plan should be part of proposal

Kyle comment: Data in nuclear experiment and theory lies at the root of discovery and frequently remains relevant long after it's taken or produced. Mechanisms for long-term preservation of data and metadata, including research software and workflows, should be established to ensure accessibility and reproducibility of publicly funded science.

Peter comment: experience with reanalysis of archived LEP and HERA data show that strong institutional memory is crucial for effective data preservation - just the data and software, without deeper knowledge of the experiment and apparatus, is inadequate for high-quality analyses. Not clear what exactly the recommendation is on this point, but the current experience should be noted.

\subsubsection{WG slides}

Data and analysis and knowledge preservation, enabled by institutional memory, driven by workforce development. 
When appropriate, data should be preserved for future analysis or re-analysis with newly developed methods from the field of Data Science
All components used in model-to-data comparisons, including experimental data, intermediate and final model results, software, and workflows should be preserved so as to be reproducible by future researchers.
This data and metadata should be broadly and easily accessible to the community.
This includes preservation of trained AI/ML models and surrogates and detailed information of training data used to inform the models

%=======================================================

\section{Pre-workshop Overleaf text}

%---------------------------------
\subsection{Software infrastructure}

Bullets from Amber:

\begin{itemize}

\item What does Software innovation and evolution look like in the post-ECP era?

\item What Software Infrastructure is needed to support collaborative use and sustainability?

\item What Software infrastructure is need to support AI/ML development and innovation?

\item What would enable a software lifecycle that extends from innovation through retirement?  (to get at the SciDac lock-out issue)?

\end{itemize}

%---------------------------------
\subsection{Input from BAND}
\label{Sect:BAND}

Daniel Phillips email to Amber and Peter April 28: There are three topics we in BAND would like to see discussed at the workshop. These topics are not scientific topics per se, but they absolutely have to do with existing barriers to establishment of effective software infrastructure in nuclear physics.

\subsubsection{Design environment}
 
The software design environment. We need to design environments for building scientific software that help students + post-docs (+ faculty!) learn how to build sustainable, extensible, well-coded software. Such environments should include good materials for onboarding, methods for communication between team members etc. Github has become a bit of a standard in our community and it does many of these things well. But the three of us talked about the strategic vulnerability that results from relying on Microsoft’s business model not changing, such that features we really on in GitHub go away. 

It might be worth thinking about the ways in which a research software environment differs from one used to build a commercial product, and what such an environment might look like if we built it from the ground up, using, say, free git tools rather than relying on their implementation per Microsoft (or someone else).

\subsubsection{Workforce}

Software sustainability and career paths that facilitate that. Sustainability of scientific software is a big problem. If a software suite becomes popular enough then a community of developers will ensure it continues to run as new O/Ses come out, and that issues with broken dependencies get remedied, bugs get fixed, etc. But while this might work for bumpy it is not a realistic hope for most scientific software. 

Who fixes bugs and delivers desired feature enhancements once the graduate student who wrote the initial version of the software has moved on? Our field has not traditionally provided good career opportunities for Research Software Engineers. But if we are going to have good Software Infrastructure such folks are surely essential, just as specialists on instrumentation, DAQ, etc. are essential to experimental infrastructure. Is it unhealthy if all our field’s RSEs sit at National Labs, and software that is initially built with university involvement is ultimately maintained through labs? What can we do to encourage universities to provide career paths for RSEs? Thinking more generally, what culture shift is needed to encourage universities to hire and promote scientists whose main gift is turning ideas into efficient code?

\subsubsection{Data integrity}

Data integrity and reproducibility of results. How do we ensure that software comes with a test suite? And runs accurately on different platforms? Where is the data from big scientific computing enterprises going to be stored? How public will it be? 

I do want to add that on \#1 and \#2 I think the pivotal moment that we are at means that we have an opportunity to shift our field's culture so that people coming into the field understand good software practices better than their predecessors did. But the code-development environment and the field’s incentive structure will shape that culture, so we should do what we can to get those right. As Amber said, we can frame this as innovating the environment, and our practices, and thereby placing us better for long-term success in this software-driven world.

Lastly we talked about the fact that the CSSI program has been wrestling with some of these issues for some time, and it could be useful to have their input so we benefit from solutions they have found, or tried and found wanting, to these issues.
